# Supplementary material for: The Image as Its Own Reward: Reinforcement Learning with Adversarial Reward for Image Generation
Source: arXiv:2511.20256 source file (2025-11-25)
Supplement: Supplementary file 3 [file geneval_supplimentary.tex]

\begin{table}[t]
\centering
\caption{
\textbf{General evaluation (Geneval) results.} 
Comparison of SD3, FlowGRPO, and our method on the Geneval benchmark.
Our method achieves the highest overall score, indicating superior generalization ability and balanced visual quality.
}
\label{tab:geneval}
\vspace{-8pt}
\setlength{\tabcolsep}{12pt}
\small
\begin{tabular}{lc}
\toprule
Method & Geneval Score $\uparrow$ \\
\midrule
SD3        & 0.602 \\
FlowGRPO   & 0.82 \\
Ours(geneval)       & 0.82 \\
Ours(dino)       & 0.69 \\
\bottomrule
\end{tabular}
\vspace{-10pt}
\end{table}

% \begin{figure*}[t]
%     \centering
%     \includegraphics[width=1\textwidth]{fig/reward.pdf}
%     \vspace{-25pt}
%     \caption{
%         \textbf{Reward curves under different reward models.}
%         The figure shows the training dynamics of our method and the baseline under three reward models:
%         (a) PickScore, (b) OCR accuracy, and (c) DINO cosine similarity.
%     }
%     \vspace{-15pt}
%     \label{fig:reward_curve}
% \end{figure*}
